# Supplementary material for: Matched sample selection with GANs for mitigating attribute confounding
Source: arXiv:2103.13455 source file (2021-03-24)
Supplement: Supplementary file 1 [file supp_broader_impacts.tex]

\section*{Broader impacts}

It is critically important to consider the use-cases of facial recognition technology. It is being used across the world to surveil and explicitly discriminate against minority groups. Moreover, systems employing facial recognition regularly discriminate implicitly against minority groups in a variety of settings, from judging personality to interview screening. These issues are all urgently important and cannot be solved with statistical measures of fairness. %They require systematic opposition by the computer vision community.

The work here in no way condones any such use of facial recognition technology. At a minimum, the authors hope that the work here recommends caution in the deployment of any system employing facial recognition technology. Even with a very careful evaluation of the possible biases present in a system, as this work proposes, the context and implications of the system must be weighed with deliberate scrutiny. In many cases, a solution is to avoid using facial recognition technology rather than try to mitigate its bias.

In addition, different entities developing and using facial recognition technology have infringed heavily on the privacy of individuals. Privacy and consent are hugely important and here we attempt to limit our part in this by using only publicly available images of celebrities.

% As previously mentioned, the work here uses labels for a celebrity's gender which were manually annotated in the curation of the CelebA dataset~\cite{liu2015faceattributes}. These annotations unfortunately assume that gender can be externally assigned and forced into binary categories. To make these potentially harmful assumptions transparent, we refer throughout to a celebrity's `perceived gender' rather than their `gender'.
We hope the tools here can help call attention to important issues surrounding bias in computer vision and forge a path towards mitigating them.
The methods here are mostly exploratory, demonstrating the utility of GAN-based matching as a tool for benchmarking bias. 
As a result, the facial-recognition analysis here is limited. The dataset considered, CelebA-HQ, consists only of high-resolution celebrity images in decent lighting conditions. 
To overcome these restrictions, we hope the techniques here enable more rigorous benchmarking on detailed datasets, likely massive private datasets which are already collected by governments (e.g. US visa application headshots~\cite{grother2019ongoing3}). Such analyses could include a wealth of metrics going beyond mean facial distance for different classifiers.
