# Supplementary material for: Matched sample selection with GANs for mitigating attribute confounding
Source: arXiv:2103.13455 source file (2021-03-24)
Supplement: Supplementary file 2 [file supp_disentanglement.tex]

\section{Disentanglement in face space}
\label{sec:disentanglement}
We want a disentangled latent space. This type of disentanglement is difficult to do automatically because datasets are biased. Paired data could solve the problem...However, this data is difficult and sometimes impossible to collect (e.g. changing gender, ethnicity). New things here: (1) explicit disentanglement, (2) focus on human annotations which avoids bias from classifiers, (3) ability to use priors, with some theoretical analysis.

\subsection{Basic setup}
We are given a latent space matrix $\zmat \in \R^{N \times N_Z}$, corresponding attributes $\amat \in \R^{N \times N_A}$ (where $N$ is the number of data points, $N_A$ the number of attributes, and $N_Z$ the size of the latent space; in our case they are 5000, 6, and 512, respectively). Our goal is to learn a mapping $T: \R^{N_Z} \to \R^{N_A}$, producing predictions $T(\zmat) = \hat \amat \in \R^{N \times N_A}$. 

\paragraph{Orthogonalization setup} Standard practice aims to minimize the prediction error of each using a linear model. For each attribute $j$, one minimizes the prediction error of the corresponding column $||\amat_{, j} - \hat \amat_{, j}||^2_F$. This is usually done for a linear model (e.g. $T(\zmat) = \wmat \zmat$). To ensure independence, studies then orthogonalize the directions learned by each linear model, i.e. by using the Gram-Schmidt procedure on the matrix $\wmat$~\cite{shen2019interpreting}.

\paragraph{Defining disentanglement}
A simple definition of disentanglement is that varying one attribute does not vary the others, i.e. the projections of the points onto each attribute's direction are independent. Mathematically, this amounts to saying the columns of the predictions $\mathbf{\hat{A}}$ should be independent. This disentanglement comes from two parts: (1) the correlations in this data and (2) the irreducible correlations.

\subsection{Disentanglement tradeoff}

We can make this more explicit by incorporating independence into the loss function itself. That is, we minimize the following:

\begin{equation}
    \mathcal L = \underbrace{||\amat - T(\zmat)||_F}_{\text{mean-squared error}} + \lambda \underbrace{\sum_{i=1}^{N_A} \sum_{j=0}^{i} |\rho_{i, j}|}_{\text{inter-attribute correlation}}
    \label{eq:loss_disentanglement}
\end{equation} 
where $\rho_{i, j}$ denotes the Pearson correlation between the $i$-th and $j$-th column of $\hat \amat$ and $\lambda$ is a hyperparameter which trades off the two terms.

\commentCS{Also should add inter-attribute gradient correlation. This says, changing an attribute, should not affect another attribute.}

\cref{fig:attr_mse} varies $\lambda$ and shows the results. Data consists of 5,000 randomly sampled synthetic images from StyleGAN2, and each of the 6 attributes is annotated and averaged over 7 annotators. 3,500 images are used for training, 1,500 for testing. Here, ``MLP'' refers to a simple 3-layer fully connected neural network with hidden size of 100 and `INN' refers to an invertible neural network using 8 GLOW blocks, implemented in FreIA\footnote{https://github.com/VLL-HD/FrEIA}.

\paragraph{Latent space priors}

Some correlations are unavoidable (e.g. young/old and long hair)....so we can put them in explicitly. We can also weight the correlations that we care the most about. This can be done by manually specifying a groundtruth replacing the $|\rho_{i, j}|$ term in \cref{eq:loss_disentanglement} with a term $|\rho_{i, j} - \rho^{\star}_{i, j}|$, where $\rho^{\star}_{i, j}$ is a groundtruth correlation which is known. Moreover, such groundtruth correlations can be specified for only subsets of the values of an attribute (e.g. babies with very long hair).

\begin{figure}[H]
    \centering
    \includegraphics[width=0.8\textwidth]{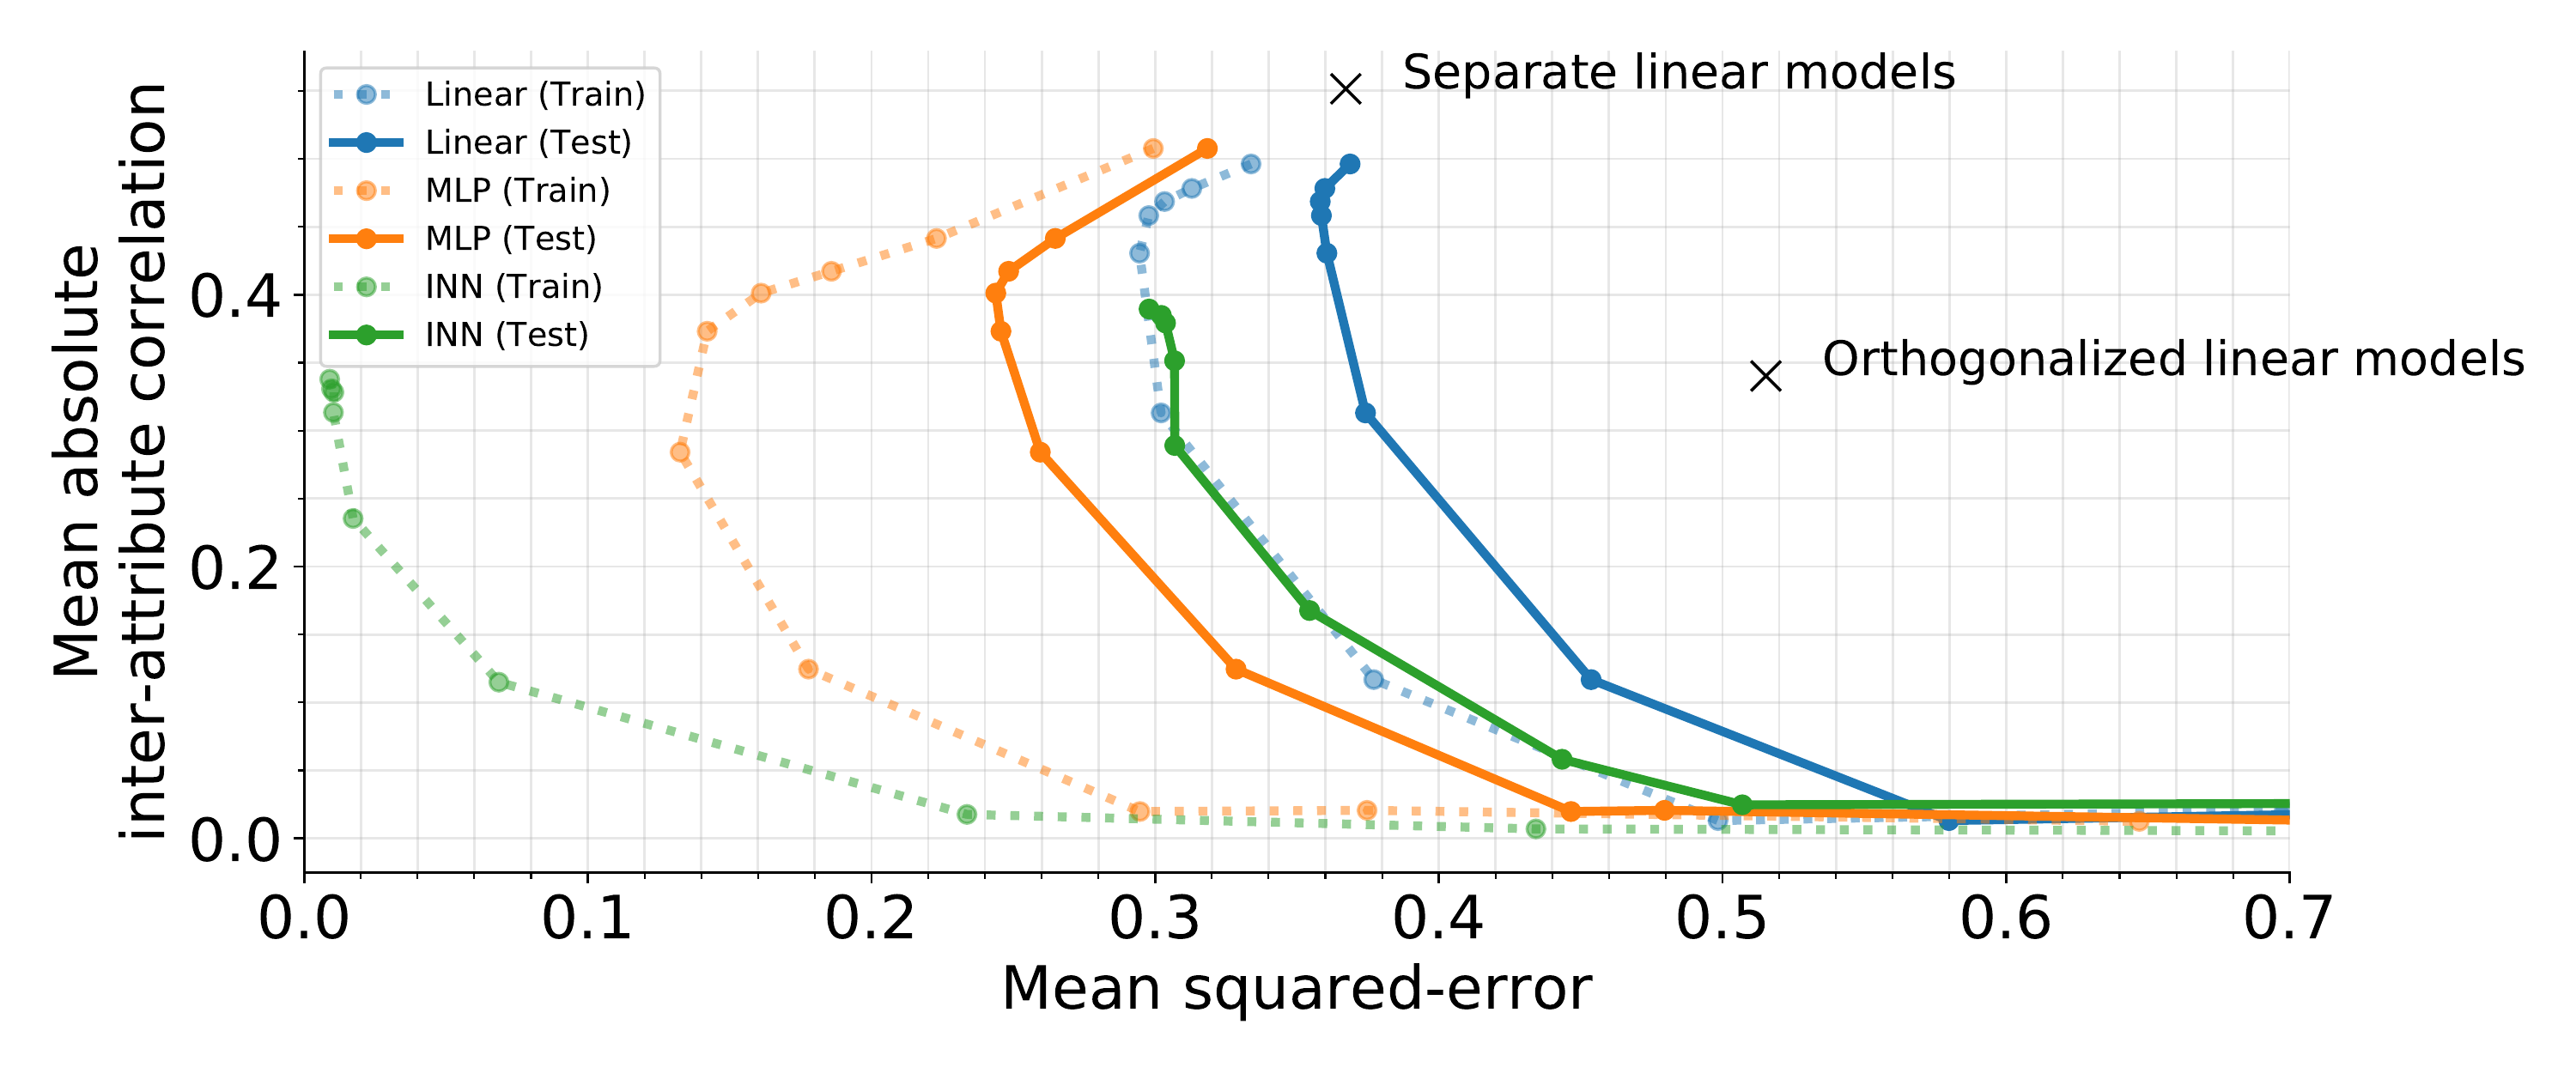}
    \caption{Penalizing inter-attribute correlation can simultaneously minimize the correlations and the mean-squared error for testing data. Non-linear model is also able to outperform linear model. Results hold for spearman correlation as well as MSE.}
    \label{fig:attr_mse}
\end{figure}

The attributes used for orthogonalization are these 6: `age', `facial-hair', `skin-color', `gender', `hair-length', and `makeup'.

We then train our model on the full dataset (5,000 + 8,000) images. To avoid potential issues (e.g. not enough data, noise vars in INN could be correlated), we use linear model.

\paragraph{Work on non-linear mappings of latent space}
Most similar to the work here is this approach which uses an invertible neural network to map latent space to interpreteable feature space~\cite{esser2020disentangling}. Main difference is that their setting does not focus on annotation, rather each attribute is learned relatively unsupervised and a single concept can be represented by many latent dimensions, making it hard to parse.

Related previous work uses different directions for semantic face editing \cite{shen2019interpreting, shen2020interfacegan}. However, these directions are linear, not jointly learned, and orthogonalized in the latent space.

\paragraph{Qualitative results} Generated images...

\paragraph{Can we independently vary an attribute} Human experiment showing that we can independently vary an attribute on image pairs that have only slight modification. Generate a bunch of random images, alter only one attribute, collect human annotations for each of the attributes. Then, see if we can 

\subsection{Theoretical tradeoff}
% \paragraph{Theoretical tradeoff} 
\commentCS{Will work on this later...this theoretical limit is pretty impractical}

This can be measured via the rank of the matrix, or it smallest singular value: $\sigma_{\min}(\mathbf{\hat{A}})$ (the smaller it is, the less independent they are). However, this will directly trade off with the mean-squared error as defined above whenever $\mathbf A$ has attributes which are correlated. In fact, it is difficult even to benchmark disentanglement in this setup. This makes intuitive sense - some attributes can not be disentangled, i.e. they have a causal relationship and therefore one cannot be varied independently of the other. However, when they simply correlate with one another, the problem can be mitigated.

Let $\sigma_{\min}(\mathbf{A}) = 0$ (a singular matrix) and $\sigma_{\min}(\hat \amat) = \sigma$. Then, $||\amat - \hat \amat||^2_F > 0$...

How does this work for test data...?
