# Supplementary material for: Matched sample selection with GANs for mitigating attribute confounding
Source: arXiv:2103.13455 source file (2021-03-24)
Supplement: Supplementary file 3 [file supp_fixing_bias.tex]

\section{Fixing bias}

\begin{figure}[H]
    \centering
    \includegraphics[width=\textwidth]{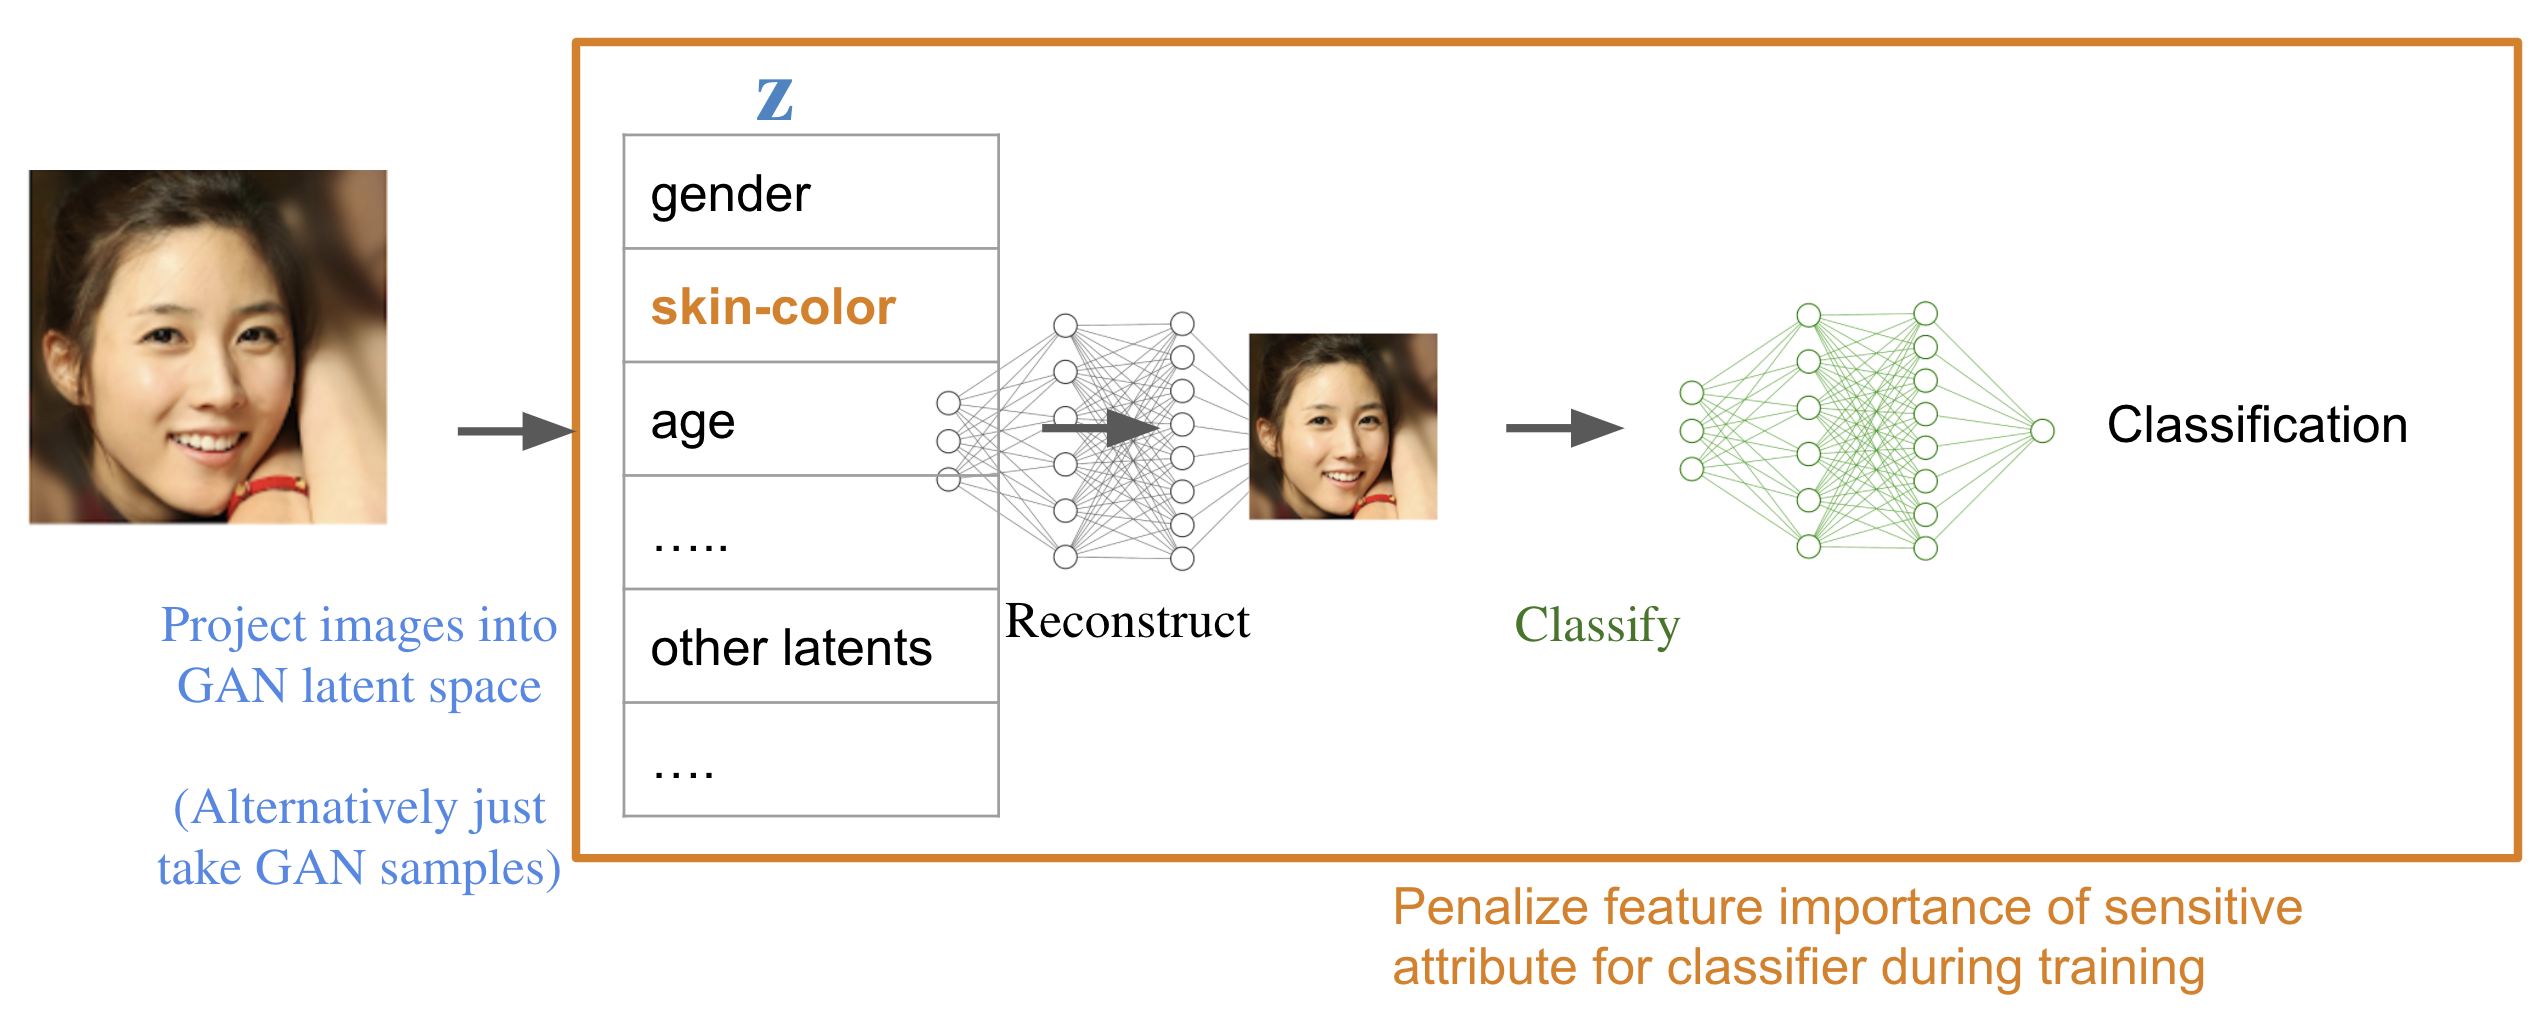}
    \caption{Fixing bias proposal}
    \label{fig:fixing_bias}
\end{figure}
